# Supplementary material for: The kernel-balanced equation for deep neural networks
Source: arXiv:2309.07367 source file (2023-09-14)
Supplement: Supplementary file 1 [file appendix1.tex]

\section{Response Kernel Dynamics} \label{sec:appendix}
Here we analyse response kernel dynamics,
\begin{equation}
\frac{d\bm{y_i}}{dt}=K(\bm{y}^*_i-\bm{y}_i),
\end{equation}
where each variable, $\bm{y}_i$, is converged into the target one, $\bm{y}^*_i$.
To be noted, we focus on short term dynamics and ignore aging in the training response for simplicity.
We can write it in another form,
\begin{equation}
\frac{d\bm{z}_i}{dt}=-K\bm{z}_i,
\end{equation}
where the error, $\bm{z}_i$, is used as the replacement of the original variable, $\bm{y}_i$.
The kernel matrix, $K$, depends on the distance on the input space, $\bm{x}_i$,
\begin{equation}
K_{ij}=K(|\bm{x}_i-\bm{x}_j|)\sim\exp(-\alpha|\bm{x}_i-\bm{x}_j|).
\end{equation}
We can show the eigen vectors of the matrix, $K$, have a localized wave-like form. The eigen values are reduced for the case of narrower waves. In other words, errors with larger scale should diminish soon, but ones with smaller scale require longer time to be diminished. We show the dynamics of error in the frequency domain in the figure \ref{fig:error_dyn}.
\begin{eqnarray}
\frac{d\bm{y}_i}{dt}&=&-\sum_jK_{ij}(\bm{y}_j-\bm{y}^*_j)\\
&\sim&\sum_k\lambda_k\sum_j\Tilde{K}_{ijk}(\bm{y}_j^*-\bm{y}_j)\\
&\sim&\sum_k\lambda_k\sum_j\Tilde{K}_{ijk}(\bm{y}_j^*-\bm{y}_i)
\end{eqnarray}
